# Supplementary material for: A program logic for fresh name generation
Source: arXiv:2101.10720 source file (2021-03-12)
Supplement: Supplementary file 1 [file appendix_reasoning.tex]

\subsection{\color{green}$M_{c1} \equiv \LET{x}{\GENSYM()}{\lambda y.x = y}$}

\PROOFFINISHED
{
	\begin{NNDERIVATION}{1}
%		\label{reasoning_canonical}
		\NLINE{\GAMMA \PLUSV x \PLUSTC \TCV \PLUSV y \Vdash 
			\ASSERT
			{\TRUTH}
			{x = y}{m}
			{m = (\EQA{x}{y})}}
		{\RULENAME{Eq}}
		\NLINE{\GAMMA \PLUSV x  \Vdash 
			\ASSERT
			{\TRUTH}
			{\lambda y.x = y}{u}
			{\FAD{\TCV}\FORALL{y}{\TCV} \ONEEVAL{u}{y}{m}{m = (\EQA{x}{y})}}
		}{\RULENAME{Lam}, 1}
		\NLINE{\GAMMA \PLUSV x  \Vdash 
			\ASSERT
			{\FRESH{x}{\GAMMA}}
			{\lambda y.x = y}{u}
			{\FRESH{x}{\GAMMA} \PAND  \FAD{\TCV}\FORALL{y}{\TCV}\ONEEVAL{u}{y}{m}{m = (\EQA{x}{y})}}
		}{\RULENAME{Invar}, 2}
		\NLINE{
			\begin{array}[t]{l}	
				\FRESH{x}{\GAMMA} \PAND \FAD{\TCV}\FORALL{y}{\TCV} \ONEEVAL{u}{y}{m}{m = (\EQA{x}{y})}
				\\
				\PIMPLIES \ 
				\FORALL{y}{\GAMMA \PLUSV u} \ONEEVAL{u}{y}{m}{m = \FALSE}
			\end{array}
		}{see below, Line 7}
		\NLINE{\GAMMA \Vdash 
			\ASSERT
			{\TRUTH}
			{M_{c1}}{u}
			{\FORALL{y}{\GAMMA \PLUSV u} \ONEEVAL{u}{y}{m}{m = \FALSE}}
		}{ \RULENAME{LetFresh}}
		\NLASTLINE{\GAMMA \Vdash 
			\ASSERT
			{\TRUTH}
			{M_{c1}}{u}
			{\FAD{\TCV}\FORALL{y^{\NAME}}{\TCV} \ONEEVAL{u}{y}{m}{m = \FALSE}}
		}{Ax (utc2)}
	\end{NNDERIVATION}
	
	To prove $
	\begin{array}[t]{l}	
		\FRESH{x}{\GAMMA} \PAND \FAD{\TCV}\FORALL{y}{\TCV} \ONEEVAL{u}{y}{m}{m = (\EQA{x}{y})}
		\\
		\PIMPLIES \ 
		\FORALL{y}{\GAMMA \PLUSV u} \ONEEVAL{u}{y}{m}{m = \FALSE}
	\end{array}$
	\\ 
	see the following:
	\PROOFFINISHED{
		\begin{NDERIVATION}{7}
			\NLINE{\GAMMA \PLUSV x \PLUSV u  \Vdash 
				\FRESH{x}{\GAMMA} \PAND \FAD{\TCV}\FORALL{y}{\TCV} \ONEEVAL{u}{y}{m}{m = (\EQA{x}{y})}	
			}{}
			\NLINE{\MIMPLIES \ \GAMMA \PLUSV x \PLUSV u  \Vdash 
				\FRESH{x}{\GAMMA} \PAND \FORALL{y}{\GAMMA \PLUSV x \PLUSV u} \ONEEVAL{u}{y}{m}{m = (\EQA{x}{y})}	
			}{Ax (utc1)}
			\NLINE{\MIMPLIES \ \GAMMA \PLUSV x \PLUSV u  \Vdash { 
					\FRESH{x}{\GAMMA \PLUSV u} \PAND \FORALL{y}{\GAMMA \PLUSV x \PLUSV u} \ \ONEEVAL{u}{y}{m}{m = (\EQA{x}{y})}}
			}{Ax (f1)}
			\NLINE{\MIMPLIES \ \GAMMA \PLUSV x \PLUSV u  \Vdash 
				\FRESH{x}{\GAMMA \PLUSV u} \PAND \FORALL{y}{\GAMMA \PLUSV u} \ \ONEEVAL{u}{y}{m}{m = (\EQA{x}{y})}
			}{Ax (u2)}
			\NLINE{\MIMPLIES \ \GAMMA \PLUSV x \PLUSV u  \Vdash 
				\FORALL{y}{\GAMMA \PLUSV u} \ \FRESH{x}{\GAMMA \PLUSV u \PLUSV y} \PAND \ONEEVAL{u}{y}{m}{m = (\EQA{x}{y})}
			}{Ax (f2)}
			\NLINE{\MIMPLIES \ \GAMMA \PLUSV x \PLUSV u  \Vdash 
				\FORALL{y}{\GAMMA \PLUSV u} \ x \neq y \PAND \ONEEVAL{u}{y}{m}{m = (\EQA{x}{y})}
			}{Ax (f3)}
			\NLASTLINE{\MIMPLIES \ \GAMMA \PLUSV x \PLUSV u  \Vdash 
				\FORALL{y}{\GAMMA \PLUSV u} \ONEEVAL{u}{y}{m}{m = \FALSE}
			}{Ax (e4)}
		\end{NDERIVATION}
	}
}

\subsection{\color{green} $M_{c2} \equiv \LET{x}{\GENSYM()}{\PAIR{x}{\lambda y.x = y}}$}
A similar proof to Sec \ref{reasoning_canonical} holds for the inner $\lambda y. x=y$, with the exception that Ax (utc2) fails i.e. 
$\ASSERT
{\TRUTH}
{M_{c1}}{u}
{\FORALL{y}{\GAMMA \PLUSV u} \ONEEVAL{u}{y}{m}{m = \FALSE}}$ 
holds but this is too restrictive, as it states nothing about $\ONEEVAL{u}{x}{m}{...}$. A more general assertion is derived stating the cases for $\pi_2(M_{c2})$ applied to both $\pi_1(M_{c2})$ and any other name.
\PROOFFINISHED
{
	\begin{NDERIVATION}{1}
		\NLINE{\text{Let: } C(p,q) \equiv \FRESH{p}{\GAMMA} \PAND \FAD{\TCV}\FORALL{y}{\TCV} \ONEEVAL{q}{y}{d}{d = (\EQA{p}{y})}}{}
		\NLINE{\GAMMA \PLUSV x \Vdash 
			\ASSERT
			{\FRESH{x}{\GAMMA}}
			{x}{b}
			{x=b \PAND \FRESH{x}{\GAMMA}}
		}{\RULENAME{Var}}
		
		\NLINE{\GAMMA \PLUSV x \PLUSV b  \Vdash 	
			\ASSERT
			{\TRUTH}
			{\lambda y.x = y}{c}
			{\FAD{\TCV}\FORALL{y}{\TCV} \ONEEVAL{c}{y}{d}{d = (\EQA{x}{y})}}
		}{Sec \ref{reasoning_canonical} lines 1-3}
		\NLINE{\GAMMA \PLUSV x \PLUSV b  \Vdash
			\ASSERT
			{x=b \PAND \FRESH{x}{\GAMMA}}
			{\lambda y.x = y}{c}
			{
				x=\pi_1(\PAIR{b}{c}) \PAND C(x,c)
			}
		}{\RBOX{
				\RULENAME{Conseq}, \RULENAME{Invar}, 3
		}}
		\NLINE{
			\GAMMA \PLUSV x \PLUSV b  \Vdash
			\ASSERT
			{x=b \PAND \FRESH{x}{\GAMMA}}
			{\lambda y.x = y}{c}
			{C(\pi_1(a), \pi_2(a)) \LSUBST{\PAIR{b}{c}}{a}}
		}{\RULENAME{Conseq}, Ax (eq4)}
		\NLINE{\GAMMA \PLUSV x  \Vdash 
			\ASSERT
			{\FRESH{x}{\GAMMA}}
			{\PAIR{x}{\lambda y.x = y}}{a}
			{C(\pi_1(a), \pi_2(a))}
		}{\RULENAME{Pair}, 1, 5}
		\NLASTLINE{\GAMMA \Vdash 
			\ASSERT
			{\TRUTH}
			{M_{c2}}{a}
			{\FRESH{\pi_1(a)}{\GAMMA} \PAND \FAD{\TCV}\FORALL{y}{\TCV} \ONEEVAL{\pi_2(a)}{y}{d}{d = (\EQA{\pi_1(a)}{y})}}
		}{\RBOX{ 
				\RULENAME{LetFresh}, 6
			}
		}
	\end{NDERIVATION}
	
}

\subsection{\color{green}$F_1'(n_0) \equiv \lambda x. \IFTHENELSE{x=n_0}{n_1}{n_0}$ in $F_1(n_0) = \LET{n_0,n_1}{\GENSYM()}{F_1'(n0)}$}

\PROOFFINISHED
{
	\begin{NNDERIVATION}{1}
		\NLINE{
%			\GAMMA \PLUSV x \PLUSTC \TCV \PLUSV y \Vdash 
			\ASSERT
			{\EQA{x}{n_0}}
			{x=n_0}{b}
			{b = \TRUE}
		}{\RULENAME{Eq}}
		\NLINE{
%			\GAMMA \PLUSV x \PLUSTC \TCV \PLUSV y \Vdash 
			\ASSERT
			{\TRUE = \TRUE}
			{n_1}{c}
			{c=n_1}
		}{\RULENAME{Const}}
		\NLINE{
%			\GAMMA \PLUSV x \PLUSTC \TCV \PLUSV y \Vdash 
			\ASSERT
			{\FALSE = \TRUE}
			{n_0}{c}
			{c=n_0}
		}{\RULENAME{Const}}
		\NLINE{
%			\GAMMA \PLUSV x \PLUSTC \TCV \PLUSV y \Vdash 
			\ASSERT
			{\TRUTH}
			{n_0}{c}
			{\FALSITY \PIMPLIES c=n_0}
		}{\RULENAME{$\PAND-\PIMPLIES$}}
		\NLINE{
%			\GAMMA \PLUSV x \PLUSTC \TCV \PLUSV y \Vdash 
			\ASSERT
			{\FRESH{n_0}{\GAMMA} \PAND\FRESH{n_1}{\GAMMA \PLUSV n_0} \PAND \EQA{x}{n_0} }
			{\IFTHENELSE{x=n_0}{n_1}{n_0}}{c}
			{c=n_1}
		}{\RULENAME{If}}
		\NLINE{
%			\GAMMA \PLUSV m \PLUSV n  \Vdash 
			\ASSERT
			{\FRESH{n_0}{\GAMMA} \PAND\FRESH{n_1}{\GAMMA \PLUSV n_0}}
			{F_1'(n_1)}{u}
			{\FAD{\TCV}\FORALL{x}{\TCV} x=n_0 \PIMPLIES \ONEEVAL{u}{x}{c}{c =n_1 }}
		}{\RULENAME{Lam}, 5}
		\NLINE{
%			\GAMMA \PLUSV m \PLUSV n  \Vdash 
			\ASSERT
			{\FRESH{n_0}{\GAMMA} \PAND\FRESH{n_1}{\GAMMA \PLUSV n_0}}
			{F_1'(n_1)}{u}
			{\ONEEVAL{u}{n_0}{c}{c =n_1}}
		}{\RULENAME{Conseq}}
		\\
		\NLINE{...}{Lines (1-4)}
		\NLINE{
%			\GAMMA \PLUSV x \PLUSTC \TCV \PLUSV y \Vdash 
			\ASSERT
			{\FRESH{n_0}{\GAMMA} \PAND\FRESH{n_1}{\GAMMA \PLUSV n_0}}
			{\IFTHENELSE{x=n_0}{n_1}{n_0}}{c}
			{c=n_0}
		}{\RULENAME{If}}
		\NLINE{
%			\GAMMA \PLUSV m \PLUSV n  \Vdash 
			\ASSERT
			{\FRESH{n_0}{\GAMMA} \PAND\FRESH{n_1}{\GAMMA \PLUSV n_0}}
			{F_1'(n_1)}{u}
			{\FAD{\TCV} \FORALL{x^{\NAME}}{\TCV} x \neq n_0 \PIMPLIES \ONEEVAL{u}{x}{c}{c =n_0}}
		}{\RULENAME{Lam}, 8}
		\NLINE{
%			\GAMMA \PLUSV m \PLUSV n  \Vdash 
			\ASSERTTALL
			{\FRESH{n_0}{\GAMMA} \PAND\FRESH{n_1}{\GAMMA \PLUSV n_0}}
			{F_1'(n_1)}{u}
			{\FRESH{n_0}{\GAMMA} \PAND\FRESH{n_1}{\GAMMA \PLUSV n_0} 
				\PAND \ONEEVAL{u}{n_0}{c}{c =n_1 } 
				\PAND \FAD{\TCV} \FORALL{x^{\NAME}}{\TCV} x \neq n_0 \PIMPLIES \ONEEVAL{u}{x}{c}{c =n_0}}
		}{\RULENAME{$\PAND$-post}, 7, 10}
		\\
		\NLINE{
			\begin{array}[t]{ll}	
				\FRESH{n_0}{\GAMMA} \PAND\FRESH{n_1}{\GAMMA \PLUSV n_0} \PAND \ONEEVAL{u}{n_0}{c}{c =n_1 } \PAND \FAD{\TCV} \FORALL{x^{\NAME}}{\TCV} x \neq n_0 \PIMPLIES \ONEEVAL{u}{x}{c}{c =n_0}
				\\
				\PIMPLIES \ 
				\EXISTS{m_0}{a} n_0=m_0 \PAND \ONEEVAL{u}{m_0}{c}{c =n_1 }
				&
				(ex2)+(ex3)
				\\
				\PIMPLIES \ 
				\EXISTS{m_0}{a} n_0=m_0 \PAND \EXISTS{m_1}{u\PLUSV m_0} m_1=n_1
				&
				(ex2)
				\\
				\PIMPLIES \ 
				(\EXISTS{m_0}{a} \EXISTS{m_1}{u\PLUSV m_0} (n_0=m_0 \PAND n_1=m_1)) \PAND ...
				&
				\text{assumption}
				\\
				\PIMPLIES \ 
				\EXISTS{m_0}{a} \EXISTS{m_1}{u\PLUSV m_0} 
				\left(
				\begin{array}{l}
					\FRESH{m_0}{\GAMMA} \PAND \FRESH{m_1}{\GAMMA \PLUSV m_0} \PAND 
					\ONEEVAL{u}{m_0}{c}{c =m_1} 
					\\
					\PAND \FAD{\TCV} \FORALL{x^{\NAME}}{\TCV} x \neq m_0 \PIMPLIES \ONEEVAL{u}{x}{c}{c =m_0}
				\end{array}
				\right)
				&\text{FOL}
			\end{array}
		}{}
		\NLINE{
%			\GAMMA \PLUSV m  \Vdash 
			\ASSERTTALL
			{\FRESH{m}{\GAMMA}}
			{\LET{n_1}{\GENSYM()}{F_1(n_0)}}{u}
			{\EXISTS{m_0}{a} \EXISTS{m_1}{u\PLUSV m_0} 
				\left(
				\begin{array}{l}
					\FRESH{m_0}{\GAMMA} \PAND \FRESH{m_1}{\GAMMA \PLUSV m_0} \PAND 
					\ONEEVAL{u}{m_0}{c}{c =m_1} 
					\\
					\PAND \FAD{\TCV} \FORALL{x^{\NAME}}{\TCV} x \neq m_0 \PIMPLIES \ONEEVAL{u}{x}{c}{c =m_0}
				\end{array}
				\right)}
		}{\RULENAME{LetFRESH}, 12}
		\NLINE{\GAMMA \Vdash 
			\ASSERTTALL
			{\TRUTH}
			{F_1(n_0)}{u}
			{\EXISTS{m_0}{a} \EXISTS{m_1}{u\PLUSV m_0} 
				\left(
				\begin{array}{l}
					\FRESH{m_0}{\GAMMA} \PAND \FRESH{m_1}{\GAMMA \PLUSV m_0} \PAND 
					\ONEEVAL{u}{m_0}{c}{c =m_1} 
					\\
					\PAND \FAD{\TCV} \FORALL{x^{\NAME}}{\TCV} x \neq m_0 \PIMPLIES \ONEEVAL{u}{x}{c}{c =m_0}
				\end{array}
				\right)}
		}{ \RULENAME{LetFresh}, 13}
	\end{NNDERIVATION}
}

\subsection{\color{green}$F_0'(\GENSYM()) \equiv \lambda x. \IFTHENELSE{x=n_0}{n_0}{\GENSYM()}$ in $F_0(n_0) = \LET{n_0}{\GENSYM()}{F_0'(\GENSYM())}$}
\label{app_reasoning_loop_0}
i.e.  $F_0(n_0) \equiv \LET{n_0}{\GENSYM()}{\lambda x. \IFTHENELSE{x=n_0}{n_0}{\GENSYM()}}$
\PROOFFINISHED
{
	\begin{NNDERIVATION}{1}
		\NLINE{
			%			\GAMMA \PLUSV x \PLUSTC \TCV \PLUSV y \Vdash 
			\ASSERT
			{\EQA{x}{n_0}}
			{x=n_0}{b}
			{b = \TRUE}
		}{\RULENAME{Eq}}
		\NLINE{
			%			\GAMMA \PLUSV x \PLUSTC \TCV \PLUSV y \Vdash 
			\ASSERT
			{\TRUE = \TRUE}
			{n_0}{c}
			{c=n_0}
		}{\RULENAME{Const}}
		\NLINE{
			%			\GAMMA \PLUSV x \PLUSTC \TCV \PLUSV y \Vdash 
			\ASSERT
			{\FALSE = \TRUE}
			{\GENSYM()}{c}
			{\FRESH{c}{\GAMMA \PLUSV...}}
		}{\RULENAME{Const}}
		\NLINE{
			%			\GAMMA \PLUSV x \PLUSTC \TCV \PLUSV y \Vdash 
			\ASSERT
			{\TRUTH}
			{\GENSYM()}{c}
			{\FALSITY \PIMPLIES \FRESH{c}{\GAMMA \PLUSV...}}
		}{\RULENAME{$\PAND-\PIMPLIES$}}
		\NLINE{
			%			\GAMMA \PLUSV x \PLUSTC \TCV \PLUSV y \Vdash 
			\ASSERT
			{\FRESH{n_0}{\GAMMA} \PAND \EQA{x}{n_0} }
			{\IFTHENELSE{x=n_0}{n_0}{\GENSYM()}}{c}
			{c=n_0}
		}{\RULENAME{If}}
		\NLINE{
			%			\GAMMA \PLUSV m \PLUSV n  \Vdash 
			\ASSERT
			{\FRESH{n_0}{\GAMMA}}
			{F_0'(\GENSYM())}{u}
			{\FAD{\TCV}\FORALL{x}{\TCV} x=n_0 \PIMPLIES \ONEEVAL{u}{x}{c}{c =n_0 }}
		}{\RULENAME{Lam}, 5}
		\NLINE{
			%			\GAMMA \PLUSV m \PLUSV n  \Vdash 
			\ASSERT
			{\FRESH{n_0}{\GAMMA}}
			{F_0'(\GENSYM())}{u}
			{\EVALFORMULASHORT{u}{n_0}{n_0}}
		}{\RULENAME{Conseq}}
		\\
		\NLINE{
			%			\GAMMA \PLUSV x \PLUSTC \TCV \PLUSV y \Vdash 
			\ASSERT
			{x \neq n_0}
			{x=n_0}{b}
			{b = \FALSE}
		}{\RULENAME{Eq}}
		\NLINE{
			%			\GAMMA \PLUSV x \PLUSTC \TCV \PLUSV y \Vdash 
			\ASSERT
			{\TRUE = \FALSE}
			{n_0}{c}
			{c=n_0}
		}{\RULENAME{Const}}
		\NLINE{
			%			\GAMMA \PLUSV x \PLUSTC \TCV \PLUSV y \Vdash 
			\ASSERT
			{\TRUTH}
			{n_0}{c}
			{\FALSITY}
		}{\RULENAME{Const}}
		\NLINE{
			%			\GAMMA \PLUSV x \PLUSTC \TCV \PLUSV y \Vdash 
			\ASSERT
			{\FALSE = \FALSE}
			{\GENSYM()}{c}
			{\FRESH{c}{\GAMMA \PLUSV n_0 \PLUSTC \TCV \PLUSV ...}}
		}{\RULENAME{Const}}
		\NLINE{
			%			\GAMMA \PLUSV x \PLUSTC \TCV \PLUSV y \Vdash 
			\ASSERT
			{\FRESH{n_0}{\GAMMA} \PAND x \neq n_0}
			{\IFTHENELSE{x=n_0}{n_0}{\GENSYM()}}{c}
			{\FRESH{c}{\TCV}}
		}{\RULENAME{If}}
		\NLINE{
			%			\GAMMA \PLUSV m \PLUSV n  \Vdash 
			\ASSERT
			{\FRESH{n_0}{\GAMMA}}
			{F_0'(\GENSYM())}{u}
			{\FAD{\TCV} \FORALL{x^{\NAME}}{\TCV} x \neq n_0 \PIMPLIES \ONEEVAL{u}{x}{c}{\FRESH{c}{\TCV}}}
		}{\RULENAME{Lam}, 8}
		\NLINE{
			%			\GAMMA \PLUSV m \PLUSV n  \Vdash 
			\ASSERT
			{\FRESH{n_0}{\GAMMA}}
			{F_0'(\GENSYM())}{u}
			{
				\FRESH{n_0}{\GAMMA} 
				\PAND \EVALFORMULASHORT{u}{n_0}{n_0 } 
				\PAND \FAD{\TCV} \FORALL{x^{\NAME}}{\TCV} x \neq n_0 \PIMPLIES \ONEEVAL{u}{x}{c}{\FRESH{c}{\TCV}}
			}
		}{\RULENAME{$\PAND$-post}, 7, 10}
		\NLINE{\GAMMA \Vdash 
			\ASSERT
			{\TRUTH}
			{F_0(\GENSYM())}{u}
			{...}
		}{ \RULENAME{LetFresh}, 13}
	\end{NNDERIVATION}

\[
\ONEPREMISERULENAMEDRIGHT{
	\ASSERT
	{\FRESH{n_0}{\GAMMA}}
	{F_0'(\GENSYM())}{u}
	{
		\FRESH{n_0}{\GAMMA} 
		\PAND \EVALFORMULASHORT{u}{n_0}{n_0 } 
		\PAND \FAD{\TCV} \FORALL{x^{\NAME}}{\TCV} x \neq n_0 \PIMPLIES \ONEEVAL{u}{x}{c}{\FRESH{c}{\TCV}}
	}
}{
	\ASSERT
	{\TRUTH}
	{F_0(\GENSYM())}{u}
	{...}
}{
LetFRESH
}
\]
}
