# Supplementary material for: A program logic for fresh name generation
Source: arXiv:2101.10720 source file (2021-03-12)
Supplement: Supplementary file 2 [file features_of_ATCs.tex]

\begin{definition}[Remove TCV's from ATC]
	\label{def:remove_TCV_from_ATC} \ \\
	Define a function that removes all TCVs from a ATC and leaves an ATC as follows:
	\[
	\begin{array}{ll} 
		\emptyset \REMOVETCV & \equiv \emptyset
		\\
		(\GAMMA \PLUSV x:\alpha_x) \REMOVETCV &  \equiv \GAMMA \REMOVETCV  \PLUSV x:\alpha_x
		\\
		(\GAMMA \PLUSTC \TCV:\TC) \REMOVETCV &  \equiv \GAMMA \REMOVETCV
		\\
		(\GAMMA \PLUSTC \TCV':\TC) \REMOVETCV &  \equiv \GAMMA \REMOVETCV
		\\
		(\GAMMA \PLUSG \GAMMA') \REMOVETCV &  \equiv (\GAMMA \REMOVETCV) \PLUSG (\GAMMA' \REMOVETCV)
	\end{array}
	\]
	
\end{definition}

Define a method to restrict an ATC, $\GAMMA$, from Def \ref{def:logical_language_syntax} into a typing context, $\Gamma$, from Def \ref{def:syntax}. 
The reverse is not possible as $\GAMMA$ contains order whereas $\Gamma$ does not (apart from $\emptyset$ or a single element type context).

\begin{definition}[Restricting ATCs to STCs]
	\label{def:RESTRICTATC}
	Define the restriction of an assertion typing context to a classical typing context as follows:
	\[
	\begin{array}{ll} 
		\emptyset \RESTRICTATC& \equiv \emptyset
		\\
		(\GAMMA \PLUSV x:\alpha_x) \RESTRICTATC &  \equiv \GAMMA \RESTRICTATC  ,  \ x:\alpha_x
		\\
		(\GAMMA \PLUSTC \TCV:\TC) \RESTRICTATC &  \equiv \GAMMA \RESTRICTATC
		\\
		(\GAMMA \PLUSG \GAMMA') \RESTRICTATC &  \equiv (\GAMMA \RESTRICTATC), \ (\GAMMA' \RESTRICTATC)
	\end{array}
	\]
\end{definition}

\begin{definition}[Domain of ATC]
	\label{def:ATC_domain}
	Define the domain of an ATC, $\GAMMA$, as the unordered list of variables and TCVs that occur in $\GAMMA$, written $\DOM{\GAMMA}$ and defined as follows:
	\[
	\DOM{\GAMMA} \equiv \DOM{\GAMMA\RESTRICTATC} \cup \DOM{\GAMMA\EXTRACTTC}
	\]
\end{definition}

In shorthand write $\TYPES{\GAMMA}{M}{\alpha}$ iff $\TYPES{\GAMMA\RESTRICTATC}{M}{\alpha}$.

As a dual to Def \ref{def:RESTRICTATC} define just the TCVs in a ATC.

\begin{definition}[Extracting the TCVs from an ATC]
	\label{def:EXTRACTTC}
	Define the restriction of an ATC to the TCVs as follows:
	\[
	\begin{array}{ll} 
		\emptyset \EXTRACTTC& \equiv \emptyset
		\\
		(\GAMMA \PLUSV x:\alpha_x) \EXTRACTTC &  \equiv \GAMMA \EXTRACTTC
		\\
		(\GAMMA \PLUSTC \TCV:\TC) \EXTRACTTC &  \equiv \GAMMA \EXTRACTTC \cup \{\TCV\}
		\\
		(\GAMMA \PLUSG \GAMMA') \EXTRACTTC &  \equiv (\GAMMA \EXTRACTTC)  \cup (\GAMMA' \EXTRACTTC)
	\end{array}
	\]
\end{definition}
\begin{definition}[Mapping variables in ATC's]
	\label{def:GAMMA_mapping} \ \\
	Define the type obtained by a variable in an ATC, as the function $\GAMMA( \cdot)$.
	For standard variables, $x$ (assuming $x \in \DOM{\GAMMA\RESTRICTATC}$): 
	\[
	\begin{array}{rl} 
		\emptyset(x) & \equiv \text{ error}
		\\
		(\GAMMA_0 \PLUSV x:\alpha_x) (x) &  \equiv \alpha_x
		\\
		(\GAMMA_0 \PLUSV y:\alpha_y) (x) &  \equiv \GAMMA_0 (x)
		\\
		(\GAMMA_0 \PLUSTC \TCV:\TC) (x) &  \equiv \GAMMA_0 (x)
		\\
		(\GAMMA_0 \PLUSG \GAMMA_1) (x) &  \equiv \GAMMA_0 (x) \MOR \GAMMA_1(x)  \qquad \DOM{\GAMMA_0} \cap \DOM{\GAMMA_1} = \emptyset
	\end{array}
	\]
	For TCVs, $\TCV$, it becomes more of a check of presence as opposed to a type check:
	\[
	\begin{array}{rl} 
		\emptyset(\TCV) & \equiv \text{ error}
		\\
		(\GAMMA_0 \PLUSV x:\alpha_x) (\TCV) &  \equiv \GAMMA_0(\TCV)
		\\
		(\GAMMA_0 \PLUSTC \TCV:\TC) (\TCV) &  \equiv \TC
		\\
		(\GAMMA_0 \PLUSTC \TCV':\TC) (\TCV) &  \equiv \GAMMA_0(\TCV)
		\\
		(\GAMMA_0 \PLUSG \GAMMA_1) (\TCV) &  \equiv \GAMMA_0(\TCV) \MOR \GAMMA_1(\TCV)
	\end{array}
	\]
\end{definition}

\begin{definition}[Free Variables]
	\label{def:FV_expressions} \ \\
	The \EMPH{free variables} of an expression $e$, written $\FV{e}$,  and the \EMPH{free variables} of assertions $A$, written $\FV{A}$, are defined as usual with the following additions:
	
	\[
	\begin{array}{rcl} 
		\FV{\EVALFORMULA{e}{e'}{m}{A}} & = & \FV{e} \cup \FV{e'} \cup (\FV{A}\setminus \{m\}) 
		\\
		\FV{\FRESH{x}{\GAMMA}} & = & \FV{\GAMMA} \cup  \{x\}
		\\
		\FV{\FORALL{x^{\alpha}}{\GAMMA} A} & = & (\FV{A} \setminus \{x\}) \cup \FV{\GAMMA}
		\\
		\FV{\FAD{\TCV} A} & = & \FV{A}
		\\
		\\
		\FV{\emptyset} & = & \emptyset
		\\
		\FV{\GAMMA \PLUSV x:V} & = & \FV{\GAMMA} \cup \{x\}
		\\
		\FV{\GAMMA \PLUSTC \TCV:\TC} & = & \FV{\GAMMA}
		\\
		\FV{\GAMMA \PLUSG \GAMMA'} & = & \FV{\GAMMA} \cup \FV{\GAMMA'}
	\end{array}
	\]
\end{definition}

\begin{definition}[Free Type Context Variables]
	\label{def:FTCV_expressions} \ \\
	The \EMPH{free type context variables} of assertions $A$, written $\FTCV{A}$, are defined as expected with the following additions:
	
	\[
	\begin{array}{rcl} 
		\\
		\FTCV{\EVALFORMULA{e}{e'}{m}{A}} & = & \FTCV{A}
		\\
		\FTCV{\FRESH{x}{\GAMMA}} & = & \FTCV{\GAMMA}
		\\
		\FTCV{\FORALL{x^{\alpha}}{\GAMMA} A} & = & \FTCV{A} \cup \FTCV{\GAMMA}
		\\
		\FTCV{\FAD{\TCV} A} & = & \FTCV{A} \setminus \{\TCV\}
		\\
		\\
		\FTCV{\emptyset} & = & \emptyset
		\\
		\FTCV{\GAMMA\PLUSV x:V} & = & \FTCV{\GAMMA}
		\\
		\FTCV{\GAMMA \PLUSTC \TCV:\TC} & = & \FTCV{\GAMMA} \cup \{\TCV\} 
		\\
		\FTCV{\GAMMA \PLUSTC \GAMMA'} & = & \FTCV{\GAMMA} \cup \FTCV{\GAMMA'}
	\end{array}
	\]
	\PANCHO{These may not be used and $\FTCV{\GAMMA} \equiv \GAMMA\EXTRACTTC$}
\end{definition}

The following standard abbreviations are used:

\begin{itemize}
	
	\item De Morgan dualities: 
	\begin{itemize}
		\item $A$ for $\neg \neg A$
		\item $A \OR B$ for $\neg( \neg A \AND \neg B)$
		\item $\EXISTS{x^{\alpha}}{\GAMMA} A$ for $\neg \FORALL{x^{\alpha}}{\GAMMA} \neg A$
	\end{itemize}
	
	\item $A \IFF B$ for $(A \IMPLIES B) \AND (B \IMPLIES A)$.
	
\end{itemize}

The following new abbreviations are used:

\begin{itemize}
	%  	\item $\EVALTERMINATES{x}{e}$ for $\EVALFORMULA{x}{e}{m}{\TRUTH}$. (IS THIS REQUIRED?)
	
	%  	\item $\EVALFORMULASHORT{x}{e}{e'}$ for $\EVALFORMULA{x}{e}{m}{m = e'}$, where $m$ is fresh.
	
	\item $(\GAMMA \PLUSV y)$ for $(\GAMMA \PLUSV y:\alpha)$ where $y:\alpha$ is given by the outer typing context.\\
	Specifically, where $y:\alpha$ is given by the outer typing context:
	\begin{itemize}
		\item $\FRESH{x}{\GAMMA \PLUSV y}$ for $\FRESH{x}{(\GAMMA \PLUSV y:\alpha)}$.
		\item $\FORALL{x^{\alpha}}{\GAMMA \PLUSV y} A$ for $\FORALL{x^{\alpha}}{\GAMMA \PLUSV y:\alpha} A$.	
	\end{itemize}
	
	\item $\GAMMA \PLUSTC \TCV$ as shorthand for $\GAMMA \PLUSTC \TCV:\TC$ since the variable $\TCV$ is used exclusively for type contexts of type $\TC$.
	
	%  	\item $\GAMMA \vdash \FRESH{e}{\GAMMA_0}$ for $\GAMMA \vdash \EXISTS{z}{\GAMMA} (z=e \AND \FRESH{z}{\GAMMA_0})$
	%  	\PANCHO{Is this used/required?}
	
	\item $\GAMMA \PLUSG \GAMMA'$ for $\GAMMA'$ representing an ordered mapping $x_1:\alpha_1,...,x_n:\alpha_n$ and hence $\GAMMA \PLUSG \GAMMA' \equiv ((\GAMMA \PLUSV x_1:\alpha_1) \PLUSV ....) \PLUSV x_n:\alpha_n$

\end{itemize}
