# Supplementary material for: A program logic for fresh name generation
Source: arXiv:2101.10720 source file (2021-03-12)
Supplement: Supplementary file 3 [file soundness_proof_axiom_derivable.tex]

\HIDE{
\subsubsection{\color{orange}Soundness proof of Axiom (bbSwap)}        
\[
\Gamma \vdash 
\begin{array}[t]{l}
\FORALL{x^{\NAME}}{\emptyset} \FORALL{y^{\NAME}}{\emptyset} B(x,y)
\\ \PIMPLIES \ 
\FORALL{x^{\NAME}}{\emptyset} \FORALL{y^{\NAME}}{\emptyset} B(y,x)
\end{array}
\]
NOT USED

Can be simply proven through $\alpha$-renaming
\SMALLPROOF
{
	\begin{NDERIVATION}{1}
		\NLINE{\text{Let: } \MMM^{\Gamma} \models \FORALL{x^{\NAME}}{\emptyset} \FORALL{y^{\NAME}}{\emptyset} B(x,y)}{}
		\NLINE{\text{Prove: } \MMM^{\Gamma} \models \FORALL{x}{\emptyset} \FORALL{y}{\emptyset} B(y,x)}{}
		%	\NLINE{ \IFF \forall M_x.
		%		\begin{array}[t]{l}
		%			\AN{M_x} = \emptyset
		%			\\
		%			\AND \ \TYPES{\emptyset}{M_x}{\NAME}
		%			\\
		%			\AND \ (\AN{\MMM}, M_x\MMM) \CONV (G', W_x) 
		%			\\
		%			\AND \ \MMM_x \equiv \MMM \cdot x:W_x 
		%			\\
		%			\IMPLIES \MMM_x \models \FORALL{y}{\emptyset} B(x,y)
		%		\end{array}
		%	}{}
		\NLINE{\IFF \forall M_x.
			\begin{array}[t]{l}
				\AN{M_x} = \emptyset
				\\
				\AND \ \TYPES{\emptyset}{M_x}{\NAME}
				\\
				\AND \ (\AN{\MMM}, M_x\MMM) \CONV (G', W_x) 
				\\
				\AND \ \MMM_x \equiv \MMM \cdot x:W_x 
				\\
				\IMPLIES \forall M_y.\begin{array}[t]{l}
					\AN{M_y} = \emptyset
					\\
					\AND \ \TYPES{\emptyset}{M_y}{\NAME}
					\\
					\AND \ (\AN{\MMM_y}, M_y\MMM_x) \CONV (G'', W_y) 
					\\
					\AND \ \MMM_{xy} \equiv \MMM_x \cdot y:W_y 
					\\
					\IMPLIES \MMM_{xy} \models  B(x,y)
				\end{array}
			\end{array}
		}{}
		\NLINE{ 
			\IFF
			\begin{array}[t]{l}
				M_x = \GENSYM()
				\\
				\AND \ (\AN{\MMM}, M_x) \CONV (\AN{\MMM},r_x, \ r_x) 
				\\
				\IMPLIES \begin{array}[t]{l}
					M_y= \GENSYM()
					\\
					\AND \ (\AN{\MMM},r_x,\  M_y \CONV (\AN{\MMM},r_x,r_y,\  r_y) 
					\\
					\IMPLIES \MMM \cdot x:r_x  \cdot y:r_y  \models  B(x,y)
				\end{array}
			\end{array}
		}{}
		\NLINE{ 
			\IFF
			\begin{array}[t]{l}
				M_x = \GENSYM()
				\\
				\AND \ (\AN{\MMM}, M_x) \CONV (\AN{\MMM},r_y, \ r_y) 
				\\
				\IMPLIES \begin{array}[t]{l}
					M_y= \GENSYM()
					\\
					\AND \ (\AN{\MMM},r_y,\  M_y \CONV (\AN{\MMM},r_y,r_x,\  r_x) 
					\\
					\IMPLIES \MMM \cdot x:r_y  \cdot y:r_x  \models  B(x,y)
				\end{array}
			\end{array}
		}{\RBOX{We can always swap names in the model\\ $\MMM$ is $r_x,r_y$-free \\ Lemma \ref{lem:swap_names_in_model}}}
		\NLINE{ 
			\IFF
			\begin{array}[t]{l}
				M_x = \GENSYM()
				\\
				\AND \ (\AN{\MMM}, M_x) \CONV (\AN{\MMM},r_x, \ r_x) 
				\\
				\IMPLIES \begin{array}[t]{l}
					M_y= \GENSYM()
					\\
					\AND \ (\AN{\MMM},r_x,\  M_y \CONV (\AN{\MMM},r_x,r_y,\  r_y) 
					\\
					\IMPLIES \MMM \cdot x:r_x  \cdot y:r_y  \models  B(y,x)
				\end{array}
			\end{array}
		}{\parbox[t]{5cm}{\raggedleft swap variable names in $B$
				\\
				as  $\MMM^{-r_x,r_y}$ and we know $\MMM_{xy} \models B(x,y)$ and $\SWAP{r_x}{r_y}{\MMM_{xy}} \models B(x,y)$
			}
		}
		\NLINE{ \IFF \forall M_x.
			\begin{array}[t]{l}
				\AN{M_x} = \emptyset
				\\
				\AND \ \TYPES{\emptyset}{M_x}{\NAME}
				\\
				\AND \ (\AN{\MMM}, M_x\MMM) \CONV (G', W_x) 
				\\
				\AND \ \MMM_x \equiv \MMM \cdot x:W_x 
				\\
				\IMPLIES \forall M_y.\begin{array}[t]{l}
					\AN{M_y} = \emptyset
					\\
					\AND \ \TYPES{\emptyset}{M_y}{\NAME}
					\\
					\AND \ (\AN{\MMM_y}, M_y\MMM_x) \CONV (G'', W_y) 
					\\
					\AND \ \MMM_{xy} \equiv \MMM_x \cdot y:W_y 
					\\
					\IMPLIES \MMM_{xy} \models  B(y,x)
				\end{array}
			\end{array}
		}{\RBOX{Only one option modulo excess}}
		\NLINE{\MMM^{\Gamma} \models \FORALL{x}{\emptyset} \FORALL{y}{\emptyset} B(y,x)}{Sem $\FORALL{}{}$}
	\end{NDERIVATION}
}

\subsubsection{\color{orange}Soundness proof of Axiom (bbGenSwap)}        
\ \\
\[
\Gamma,\Gamma' \vdash 
\begin{array}[t]{l}
\FORALL{x}{\Gamma} \FRESH{x}{\Gamma} \PIMPLIES \FORALL{y}{\Gamma,x} \FRESH{y}{\Gamma,x} \PIMPLIES B(x,y)
\\ \PIMPLIES \\ 
\FORALL{x}{\Gamma} \FRESH{x}{\Gamma} \PIMPLIES \FORALL{y}{\Gamma,x} \FRESH{y}{\Gamma,x} \PIMPLIES B(y,x)
\end{array}
\]
NOT USED
\SMALLPROOF
{
	\begin{NDERIVATION}{1}
		\NLINE{\text{Let: } \MMM^{\GAMMA \PLUSG \GAMMA'} \models \FORALL{x^{\NAME}}{\Gamma} \FRESH{x}{\Gamma} \IMPLIES \FORALL{y^{\NAME}}{\Gamma} \FRESH{y}{\Gamma} \IMPLIES B(x,y)}{}
		\NLINE{\text{Prove: } \MMM^{\GAMMA \PLUSG \GAMMA'} \models \FORALL{x^{\NAME}}{\Gamma} \FRESH{x}{\Gamma} \IMPLIES \FORALL{y^{\NAME}}{\Gamma} \FRESH{y}{\Gamma} \IMPLIES B(y,x)}{}
		\NLINE{ \IFF \forall M_x.
			\begin{array}[t]{l}
				\AN{M_x} = \emptyset
				\
				\AND \ \TYPES{\Gamma}{M_x}{\NAME}
				\\
				\AND \ (\AN{\MMM}, M_x\MMM) \CONV (G', W_x) 
				\\
				\AND \ \MMM_x \equiv \MMM \cdot x:W_x 
				\\
				\quad \IMPLIES \SEM{x}{\MMM_x} \notin \REACHSEMB{\Gamma}{\MMM_x} 
				\\
				\qquad \IMPLIES \MMM_x \models \FORALL{y^{\NAME}}{\Gamma} \FRESH{y}{\Gamma} \IMPLIES  B(x,y)
			\end{array}
		}{}
		\NLINE{\IFF \forall M_x.
			\begin{array}[t]{l}
				\AN{M_x} = \emptyset
				\
				\AND \ \TYPES{\Gamma}{M_x}{\NAME}
				\\
				\AND \ (\AN{\MMM}, M_x\MMM) \CONV (G', W_x) 
				\\
				\AND \ \MMM_x \equiv \MMM \cdot x:W_x 
				\\
				\quad \IMPLIES \SEM{x}{\MMM_x} \notin \REACHSEMB{\Gamma}{\MMM_x} 
				\\
				\qquad \IMPLIES \forall M_y.\begin{array}[t]{l}
					\AN{M_y} = \emptyset
					\
					\AND \ \TYPES{\Gamma}{M_y}{\NAME}
					\\
					\AND \ (\AN{\MMM_y}, M_y\MMM_x) \CONV (G'', W_y) 
					\\
					\AND \ \MMM_{xy} \equiv \MMM_x \cdot y:W_y 
					\\
					\quad \IMPLIES \SEM{y}{\MMM_{xy}} \notin \REACHSEMB{\Gamma}{\MMM_{xy}}  
					\\
					\qquad \IMPLIES \MMM_{xy} \models  B(x,y)
				\end{array}
			\end{array}
		}{}
		\NLINE{ 
			\IFF
			\begin{array}[t]{l}
				M_x = \GENSYM()
				\\
				\AND \ (\AN{\MMM}, M_x) \CONV (\AN{\MMM},r_x, \ r_x) 
				\\
				\IMPLIES \begin{array}[t]{l}
					M_y= \GENSYM()
					\\
					\AND \ (\AN{\MMM},r_x,\  M_y \CONV (\AN{\MMM},r_x,r_y,\  r_y) 
					\\
					\IMPLIES \MMM \cdot x:r_x  \cdot y:r_y  \models  B(x,y)
				\end{array}
			\end{array}
		}{}
		\NLINE{ 
			\IFF
			\begin{array}[t]{l}
				M_x = \GENSYM()
				\\
				\AND \ (\AN{\MMM}, M_x) \CONV (\AN{\MMM},r_y, \ r_y) 
				\\
				\IMPLIES \begin{array}[t]{l}
					M_y= \GENSYM()
					\\
					\AND \ (\AN{\MMM},r_y,\  M_y \CONV (\AN{\MMM},r_y,r_x,\  r_x) 
					\\
					\IMPLIES \MMM \cdot x:r_y  \cdot y:r_x  \models  B(x,y)
				\end{array}
			\end{array}
		}{\RBOX{We can always swap names in the model\\ $\MMM$ is $r_x,r_y$-free \\ Lemma \ref{lem:swap_names_in_model}}}
		\NLINE{ 
			\IFF
			\begin{array}[t]{l}
				M_x = \GENSYM()
				\\
				\AND \ (\AN{\MMM}, M_x) \CONV (\AN{\MMM},r_x, \ r_x) 
				\\
				\IMPLIES \begin{array}[t]{l}
					M_y= \GENSYM()
					\\
					\AND \ (\AN{\MMM},r_x,\  M_y \CONV (\AN{\MMM},r_x,r_y,\  r_y) 
					\\
					\IMPLIES \MMM \cdot x:r_x  \cdot y:r_y  \models  B(y,x)
				\end{array}
			\end{array}
		}{\parbox[t]{5cm}{\raggedleft swap variable names in $B$
				\\
				as  $\MMM^{-r_x,r_y}$ and we know $\MMM_{xy} \models B(x,y)$ and $\SWAP{r_x}{r_y}{\MMM_{xy}} \models B(x,y)$
			}
		}
		\NLINE{ \IFF  \forall M_x.
			\begin{array}[t]{l}
				\AN{M_x} = \emptyset
				\
				\AND \ \TYPES{\Gamma}{M_x}{\NAME}
				\\
				\AND \ (\AN{\MMM}, M_x\MMM) \CONV (G', W_x) 
				\\
				\AND \ \MMM_x \equiv \MMM \cdot x:W_x 
				\\
				\quad \IMPLIES \SEM{x}{\MMM_x} \notin \REACHSEMB{\Gamma}{\MMM_x} 
				\\
				\qquad \IMPLIES \forall M_y.\begin{array}[t]{l}
					\AN{M_y} = \emptyset
					\
					\AND \ \TYPES{\Gamma}{M_y}{\NAME}
					\\
					\AND \ (\AN{\MMM_y}, M_y\MMM_x) \CONV (G'', W_y) 
					\\
					\AND \ \MMM_{xy} \equiv \MMM_x \cdot y:W_y 
					\\
					\quad \IMPLIES \SEM{y}{\MMM_{xy}} \notin \REACHSEMB{\Gamma}{\MMM_{xy}}  
					\\
					\qquad \IMPLIES \MMM_{xy} \models  B(x,y)
				\end{array}
			\end{array}
		}{\RBOX{Only one option modulo excess}}
		\NLINE{\MMM^{\Gamma} \models \FORALL{x}{\Gamma} \FRESH{x}{\Gamma} \IMPLIES \FORALL{y}{\Gamma} \FRESH{y}{\Gamma} \IMPLIES B(y,x)}{Sem $\FORALL{}{}$}
	\end{NDERIVATION}
}
}

\HIDE{
\subsubsection{Derivable Axiom (u10):}
\ \\
$(\FORALL{x^{\alpha}}{\Gamma}(A^{-x} \OR B))  \IFF  A \OR (\FORALL{x^{\alpha}}{\Gamma}A)$

Derivable using Ax (u3), Ax (u5)
\begin{NDERIVATION}{1}
	\NLINE{\text{Assume: } \MMM \models \FORALL{x^{\alpha}}{\Gamma}(A^{-x} \OR B) }{ Let: $G=\AN{\MMM}$}
	\NLINE{\text{Prove: } \MMM \models A \OR \FORALL{x^{\alpha}}{\Gamma} B}{}
	\NLINE{\forall V.
		\begin{array}[t]{ll}
			\AN{V} = \emptyset
			&
			\AND \ \TYPES{\Gamma}{V}{\alpha}
			\\
			\AND \ (\AN{\MMM}, V\MMM) \CONV (G', W) 
			&
			\IMPLIES 
			\left(
			\begin{array}{l}
				\MMM \cdot x:W\models A^{-x} 
				\\
				\OR \ \MMM \cdot x:W\models B
			\end{array}
		\right)
		\end{array}
	}{Semantics $\FORALL{}{}$, $\AND$, 1}
	\NLINE{\forall V.
		\begin{array}[t]{ll}
			\AN{V} = \emptyset
			&
			\AND \ \TYPES{\Gamma}{V}{\alpha}
			\\
			\AND \ (\AN{\MMM}, V\MMM) \CONV (G', W) 
			&
			\IMPLIES 
			\left(
			\begin{array}{l}
				\MMM \models A 
				\\
				\OR \ \MMM \cdot x:W\models B
			\end{array}
			\right)
		\end{array}
	}{$A^{-x}$}
	\NLINE{
		\begin{array}[t]{l}
			\forall V.
			\begin{array}[t]{ll}
				\AN{V} = \emptyset
				&
				\AND \ \TYPES{\Gamma}{V}{\alpha}
				\\
				\AND \ (\AN{\MMM}, V\MMM) \CONV (G', W) 
				&
				\IMPLIES \ \MMM \models A
			\end{array}
			\\		
			\OR 
			\\ 
			\forall V.
			\begin{array}[t]{ll}
				\AN{V} = \emptyset
				&
				\AND \ \TYPES{\Gamma}{V}{\alpha}
				\\
				\AND \ (\AN{\MMM}, V\MMM) \CONV (G', W) 
				&
				\IMPLIES \ \MMM \cdot x:W \models B
			\end{array}
		\end{array}
	}{$\OR$-split}
	\NLINE{
		\MMM \models A  \OR \MMM \models \FORALL{x^{\alpha}}{\Gamma} B
	}{Inst $V$ with anything, Semantics $\FORALL{}{}$}
	\NLINE{
		\MMM \models A  \OR \FORALL{x^{\alpha}}{\Gamma} B
	}{Semantics $\OR$}
	\NLASTLINE{\text{This proof also works in reverse, as they are all $\IFF$.}}{}
\end{NDERIVATION}
}

\HIDE{
	\subsubsection{Soundness proof of Axiom (u3+u5):}
	\[
	(\FORALL{x^{\alpha}}{\Gamma}(A^{-x} \AND B))  \IFF  A \AND (\FORALL{x^{\alpha}}{\Gamma}A)
	\]
	\PANCHO{Derivable from Ax (u3)  and Ax (u5)?}
	
	\begin{NDERIVATION}{1}
		\NLINE{\text{Assume: } \MMM \models \FORALL{x^{\alpha}}{\Gamma}(A^{-x} \AND B) }{Let: $G=\AN{\MMM}$}
		\NLINE{\text{Prove: } \MMM \models A \AND \FORALL{x^{\alpha}}{\Gamma} B}{}
		\NLINE{\forall V.
			\begin{array}[t]{ll}
				\AN{V} = \emptyset
				&
				\AND \ \TYPES{\Gamma}{V}{\alpha}
				\\
				\AND \ (G, V\MMM) \CONV (G', W) 
				&
				\IMPLIES 
				\left(
				\begin{array}{l}
					\MMM \cdot x:W \models A^{-x} 
					\\
					\AND \ \MMM \cdot x:W \models B
				\end{array}
				\right)
			\end{array}
		}{Sem $\FORALL{}{}$, $\AND$, 1}
		\NLINE{
			\begin{array}[t]{ll}
				\forall V.
				\begin{array}[t]{ll}
					\AN{V} = \emptyset
					&
					\AND \ \TYPES{\Gamma}{V}{\alpha}
					\\
					\AND \ (\AN{\MMM}, V\MMM) \CONV (G', W) 
					&
					\IMPLIES 
					\left(
					\begin{array}{l}
						\MMM \cdot x:W \models A^{-x} 
						\\
						\AND \ \MMM \cdot x:W \models B
					\end{array}
					\right)
				\end{array}
				\\
				\AND
				\\
				\forall V.
				\begin{array}[t]{ll}
					\AN{V} = \emptyset
					&
					\AND \ \TYPES{\Gamma}{V}{\alpha}
					\\
					\AND \ (\AN{\MMM}, V\MMM) \CONV (G', W) 
					&
					\IMPLIES 
					\left(
					\begin{array}{l}
						\MMM \cdot x:W \models A^{-x} 
						\\
						\AND \ \MMM \cdot x:W \models B
					\end{array}
					\right)
				\end{array}
			\end{array}
		}{Duplicate}
		\NLINE{
			\begin{array}[t]{ll}
				\forall V.
				\begin{array}[t]{ll}
					\AN{V} = \emptyset
					&
					\AND \ \TYPES{\Gamma}{V}{\alpha}
					\\
					\AND \ (\AN{\MMM}, V\MMM) \CONV (G', W) 
					&
					\IMPLIES \MMM \cdot x:W \models A^{-x} 
				\end{array}
				\\
				\AND
				\\
				\forall V.
				\begin{array}[t]{ll}
					\AN{V} = \emptyset
					&
					\AND \ \TYPES{\Gamma}{V}{\alpha}
					\\
					\AND \ (\AN{\MMM}, V\MMM) \CONV (G', W) 
					&
					\IMPLIES  \MMM \cdot x:W \models B
				\end{array}
			\end{array}
		}{Remove}
		\NLINE{
			\MMM \models A 
			\ \AND \
			\forall V.
			\begin{array}[t]{ll}
				\AN{V} = \emptyset
				&
				\AND \ \TYPES{\Gamma}{V}{\alpha}
				\\
				\AND \ (\AN{\MMM}, V\MMM) \CONV (G', W) 
				&
				\IMPLIES \ \MMM \cdot x:W \models B
			\end{array}
		}{$A^{-x,V}$}
		\NLINE{
			\MMM \models A  \AND \MMM \models \FORALL{x^{\alpha}}{\Gamma} B
		}{Semantics $\FORALL{}{}$}
		\NLINE{
			\MMM \models A  \AND \FORALL{x^{\alpha}}{\Gamma} B
		}{Semantics $\AND$}
		\NLASTLINE{\text{This proof also works in reverse, as they are all $\IFF$.}}{}
	\end{NDERIVATION}
}

\HIDE{
\subsubsection{\color{green}Soundness proof of Axiom (utc77): } 
\[
	A-\text{\EXTINDEP \ } \ \MIMPLIES \ \Gamma \vdash (\FORALL{x}{\emptyset} A) \PIMPLIES \FAD{\TCV} \FORALL{x}{\Gamma,\TCV} (\FRESH{x}{\Gamma,\TCV} \PIMPLIES A)
\]
\\
\PROOFFINISHED
{
	Proof:
	\begin{NDERIVATION}{1}
		\NLINE{\text{Assume: } \MMM^{\Gamma} \models \FORALL{x}{\emptyset} A }{}
		\NLINE{\text{Prove: } \MMM^{\Gamma} \models \FAD{\TCV} \FORALL{x}{\Gamma,\TCV} (\FRESH{x}{\Gamma,\TCV} \PIMPLIES A) }{}
		\NLINE{\MMM^{\Gamma} \models \FAD{\TCV} \FORALL{x}{\emptyset} A }{Ax (utc3)}
		\NLINE{\MMM^{\Gamma} \models \FAD{\TCV} \FORALL{x}{\Gamma,\TCV} (\FRESH{x}{\Gamma,\TCV} \PIMPLIES A) }{Ax (u99)}
		
	\end{NDERIVATION}
}
}

\HIDE{

\subsubsection{\color{orange}Soundness proof of Axiom (utc3u3):} 
\[
\GAMMA \vdash A^{-\TCV} \quad \PIFF \quad  \FAD{\TCV} \FORALL{x}{\TCV} A^{-\TCV, x} \qquad  A-\EXTINDEP
\]

\PROOFFINISHED
{
	
	Derivable using Ax (u3) and Ax (utc3),
	\\
	i.e.
	$\GAMMA \vdash A \ \stackrel{Ax (u3)}{\MIFF} \ \FORALL{x}{\GAMMA} A \ \stackrel{Ax (utc3)}{\MIFF} \  \FAD{\TCV} \FORALL{x}{\GAMMA \PLUSTC \TCV} A^{-\TCV, x}$
}

}
