# Supplementary material for: A program logic for fresh name generation
Source: arXiv:2101.10720 source file (2021-03-12)
Supplement: Supplementary file 5 [file appendix_language.tex]

\section{Details of the \NUC}\label{appendix_programming_language}

Reduction contexts:

\[
\begin{array}{lll}
  \EEE{\cdot} & ::= & [\cdot ] \VERTICAL \EEE{\cdot} M \VERTICAL V \EEE{\cdot} \VERTICAL Op(\VEC{V} \EEE{\cdot} \VEC{M}) 
  \VERTICAL \IFTHENELSE{\EEE{\cdot}}{M}{N}
  \\
  & &  \VERTICAL \LET{x}{\EEE{\cdot}}{M} \VERTICAL \EEE{\cdot} = M \VERTICAL V = \EEE{\cdot}
\end{array}
\]
