# Supplementary material for: A program logic for fresh name generation
Source: arXiv:2101.10720 source file (2021-03-12)
Supplement: Supplementary file 6 [file figure_derived_rules.tex]

\begin{FIGURE}
  \begin{RULES}
        \TWOPREMISERULENAMEDRIGHT
        {
        	\begin{array}{r}
        		A, C-\text{\EXTINDEP}
        		\\
        		\MOR\ A-\text{\EXTINDEP}
        	\end{array}
        	\& \ C \THINWRT{x}
        }{
        	\GAMMA \PLUSV x:\NAME  \vdash \ASSERT{A \AND \FRESH{x}{\GAMMA}}{M}{m}{C^{-x}}
        }
        {
        	\GAMMA \vdash \ASSERT{A}{\LET{x}{\GENSYM()}{M}}{m}{C}
        }{LetFresh}
	     \\
	     \text{\PANCHO{If we can show $\FRESH{x}{\GAMMA, m}$ then we get $\EXISTS{x}{\emptyset} B$}}

  \end{RULES}
\caption{Logical rules for derived constructs. All rules are typed under $\GAMMA$.}\label{figure_derived_rules}
\end{FIGURE}
