# Supplementary material for: A program logic for fresh name generation
Source: arXiv:2101.10720 source file (2021-03-12)
Supplement: Supplementary file 7 [file further_research.tex]

\section{Further Research}

The paper \cite{BentonN:mechbisftnc} introduces the following program:
\begin{enumerate}

\item $\LET{x}{\GENSYM()}{\LET{y}{\GENSYM()}{\lambda f^{\NAME \FS
      \BOOL}. fx = fy}}$

  \item $\LET{x}{gs}{\lambda f^{\NAME \FS \BOOL}. \LET{y}{gs}{fx =
      fy}}$
\end{enumerate}
we believe that our logic cannot prove its specification. It is clear
that the logic in \cite{YHB07:local:full} can reason about both,
assuming we interpret our type $\NAME$ as $\REF{\UNIT}$ in the system
of \cite{YHB07:local:full}, and $\GENSYM$ as reference
generation. \MARTIN{Sketch why/how.} This proof makes heavy use of the
$\nu x.A$ formula of \cite{YHB07:local:full}'s.  This leaves us with
three open questions:
\begin{itemize}

\item Prove the meta-theoretic result that our logic here, more precisely
the second-order quantification XYZ, is indeed not strong enough to
deal with the examples above.

\item Do we need the full power of $\nu x.A$ for the \NUC? The
  language in \cite{YHB07:local:full} is much more powerful, including
  full higher-order state and aliasing.

  \item Would the addition of $\nu x.A$, suitably adapted, make the
  present logic observationally complete (in the sense that two
  programs are contextually indistinguishable exactly when they satisfy
  the same triples?

\end{itemize}
