# Supplementary material for: A program logic for fresh name generation
Source: arXiv:2101.10720 source file (2021-03-12)
Supplement: Supplementary file 8 [file related_works.tex]

\section{Related works}

Core works to discuss
\begin{itemize}

\item \cite{HY04PPDP}
\item \cite{YHB07:local:full}
\item \cite{BentonN:mechbisftnc}
\item Oxford work on game-theoretic semantics of \NUC
\item  Pitts / Stark work.

\end{itemize}
