# Supplementary material for: A program logic for fresh name generation
Source: arXiv:2101.10720 source file (2021-03-12)
Supplement: Supplementary file 9 [file soundness.tex]

\section{Soundness}

\begin{theorem}
All axioms and rules are sound.
\begin{proof}
	See App. \ref{sec:apndx_soundness_axioms} for soundness of axioms and App. \ref{sec:apndx_soundness_rules}for soundness of rules.
\end{proof}

\end{theorem}
